# Supplementary material for: Distance-dependent sign-reversal in the Casimir-Lifshitz torque
Source: arXiv:1801.01183 ancillary file (2018-01-03)
Supplement: Supplementary file 1 [file torba-prl-supp.pdf]

# Distance-dependent sign-reversal in the Casimir-Lifshitz torque: Supplemental material

Priyadarshini Thiyam,<sup>1,2</sup> Prachi Parashar,<sup>2</sup> K. V. Shajesh,<sup>3,2</sup> Oleksandr I. Malyi,<sup>4</sup>  
Mathias Boström,<sup>2,4</sup> Kimball A. Milton,<sup>5</sup> Iver Brevik,<sup>2</sup> and Clas Persson<sup>1,4</sup>

<sup>1</sup>*Department of Materials Science and Engineering,  
Royal Institute of Technology, SE-100 44 Stockholm, Sweden*

<sup>2</sup>*Department of Energy and Process Engineering,  
Norwegian University of Science and Technology, NO-7491 Trondheim, Norway*

<sup>3</sup>*Department of Physics, Southern Illinois University–Carbondale, Carbondale, Illinois 62901, USA*

<sup>4</sup>*Centre for Materials Science and Nanotechnology, Department of Physics,  
University of Oslo, P. O. Box 1048 Blindern, NO-0316 Oslo, Norway*

<sup>5</sup>*Homer L. Dodge Department of Physics and Astronomy,  
University of Oklahoma, Norman, Oklahoma 73019, USA*

## ON EQ. (6) AND (7)

The reduced “reflection coefficients”  $\tilde{\mathbf{R}}_i$ , for  $i = 1, 2$ , where the dependence on the degree of anisotropy  $\beta_i$  and relative orientation of two materials  $\theta$  are separated after performing the polar angle  $\phi_k$  integration in the  $k$ -space, are given by

$$\tilde{\mathbf{R}}_i = \begin{bmatrix} \frac{1}{\Delta^H} \frac{\kappa \bar{\kappa}_i^H}{(\kappa + \bar{\kappa}_i^H)^2} C_i^H & \frac{1}{\sqrt{\Delta^E \Delta^H}} \frac{2\kappa \zeta_m \kappa_i^H}{(\kappa + \bar{\kappa}_i^H)(\kappa + \bar{\kappa}_i^E)} \left( \frac{F_i}{\kappa_i^E + \kappa_i^H} - \frac{G_i}{\kappa_i^E - \kappa_i^H} \right) \\ \frac{1}{\sqrt{\Delta^E \Delta^H}} \frac{2\kappa \zeta_m \kappa_i^H}{(\kappa + \bar{\kappa}_i^H)(\kappa + \bar{\kappa}_i^E)} \left( \frac{F_i}{\kappa_i^E + \kappa_i^H} - \frac{G_i}{\kappa_i^E - \kappa_i^H} \right) & \frac{1}{\Delta^E} \frac{\kappa \zeta_m^2 \varepsilon_i^\perp}{\kappa_i^E (\kappa + \kappa_i^E)^2} C_i^E \end{bmatrix}. \quad (1)$$

The TE and TM modes do not separate in the case of the interaction between anisotropic materials. Thus,

$$\begin{aligned} \text{Tr}(\tilde{\mathbf{R}}_1 \tilde{\mathbf{R}}_2) = & \frac{1}{(\Delta^H)^2} \frac{\kappa^2 \bar{\kappa}_1^H \bar{\kappa}_2^H}{(\kappa + \bar{\kappa}_1^H)^2 (\kappa + \bar{\kappa}_2^H)^2} C_1^H C_2^H + \frac{1}{(\Delta^E)^2} \frac{\kappa^2 (\zeta_m^2 \varepsilon_1^\perp) (\zeta_m^2 \varepsilon_2^\perp)}{(\kappa + \kappa_1^E)^2 (\kappa + \kappa_2^E)^2 \kappa_1^E \kappa_2^E} C_1^E C_2^E \\ & + 2 \frac{1}{\Delta^E \Delta^H} \frac{(2\kappa)^2 \zeta_m^2 \kappa_1^H \kappa_2^H}{(\kappa + \bar{\kappa}_1^H)(\kappa + \bar{\kappa}_1^E)(\kappa + \bar{\kappa}_2^H)(\kappa + \bar{\kappa}_2^E)} \left[ \frac{F_1}{\kappa_1^E + \kappa_1^H} - \frac{G_1}{\kappa_1^E - \kappa_1^H} \right] \left[ \frac{F_2}{\kappa_2^E + \kappa_2^H} - \frac{G_2}{\kappa_2^E - \kappa_2^H} \right], \end{aligned} \quad (2)$$

where  $\Delta^E = (1 - r_1^E r_2^E e^{-2\kappa a})$  and  $\Delta^H = (1 - r_1^H r_2^H e^{-2\kappa a})$ . The reflection coefficient for the magnetic mode, for a uniaxial dielectric slab with its principal axes along  $\hat{\mathbf{z}}$  is

$$r_i^H = -\frac{\bar{\alpha}_i^H (1 - e^{-2\kappa_i^H d_i})}{1 - (\bar{\alpha}_i^H)^2 e^{-2\kappa_i^H d_i}}, \quad \bar{\alpha}_i^H = \frac{\bar{\kappa}_i^H - \kappa}{\bar{\kappa}_i^H + \kappa}. \quad (3)$$

The electric mode  $r_i^E$  is obtained by replacing  $H \rightarrow E$  in the reflection coefficient for the magnetic mode in Eq. (3). The bar on the subscript  $i$  is used to denote the rotationally symmetric uniaxial background. We have used short hand notations

$$\kappa_i^H = \sqrt{k^2 \frac{\varepsilon_i^\perp}{\varepsilon_i^n} + \frac{\zeta_m^2}{c^2} \varepsilon_i^\perp}, \quad \kappa_i^E = \sqrt{k^2 + \frac{\zeta_m^2}{c^2} \varepsilon_i^\perp}, \quad \bar{\kappa}_i^H = \kappa_i^H / \varepsilon_i^\perp, \quad \text{and} \quad \bar{\kappa}_i^E = \kappa_i^E, \quad (4)$$

where we have suppressed the explicit frequency dependence in  $\varepsilon^\perp$  and  $\varepsilon_i^n$ . The coefficients  $C_i^{H,E}$ ,  $F_i$ , and  $G_i$  are given by

$$C_i^X = \frac{\left\{ (1 - e^{-2\kappa_i^X d_i}) [1 + (\bar{\alpha}_i^X)^2 e^{-2\kappa_i^X d_i}] \mp 4\bar{\alpha}_i^X \kappa_i^X d_i e^{-2\kappa_i^X d_i} \right\}}{[1 - (\bar{\alpha}_i^X)^2 e^{-2\kappa_i^X d_i}]^2} \xrightarrow{d_i \rightarrow \infty} 1, \quad (5a)$$

$$F_i = \frac{(1 - e^{-(\kappa_i^E + \kappa_i^H) d_i}) \left( 1 - \bar{\alpha}_i^E \bar{\alpha}_i^H e^{-(\kappa_i^E + \kappa_i^H) d_i} \right)}{[1 - (\bar{\alpha}_i^E)^2 e^{-2\kappa_i^E d_i}] [1 - (\bar{\alpha}_i^H)^2 e^{-2\kappa_i^H d_i}]} \xrightarrow{d_i \rightarrow \infty} 1, \quad (5b)$$

$$G_i = \frac{(\bar{\alpha}_i^E e^{-\kappa_i^E d_i} - \bar{\alpha}_i^H e^{-\kappa_i^H d_i}) (e^{-\kappa_i^E d_i} - e^{-\kappa_i^H d_i})}{[1 - (\bar{\alpha}_i^E)^2 e^{-2\kappa_i^E d_i}] [1 - (\bar{\alpha}_i^H)^2 e^{-2\kappa_i^H d_i}]} \xrightarrow{d_i \rightarrow \infty} 0. \quad (5c)$$

Here  $X = H, E$ , and the negative and positive signs ( $\mp$ ) in the numerator of Eq. (5a) correspond to  $H$  and  $E$ , respectively.

### COMPARISON WITH EXACT UNIAXIAL RESULT

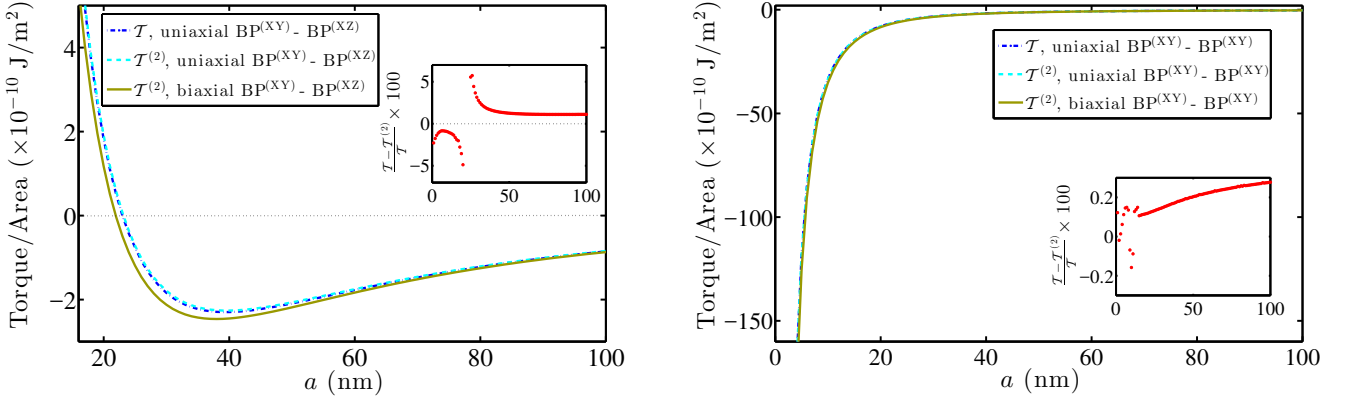

FIG. 1. Comparison between the leading-order torque  $\mathcal{T}^{(2)}$  using the perturbative theory and the total torque  $\mathcal{T}$  using the exact theory for the interaction between two uniaxial materials with optical axes in the  $u$ - $v$  plane. The left figure exhibits the interaction between nonidentical “uniaxial” materials BP<sup>(XY)</sup> and BP<sup>(XZ)</sup>, and the right panel shows the comparison for the interaction between two identical BP<sup>(XY)</sup>. The inset displays the relative percentage error, which remains well below 5% for most of the 1-100 nm range.

We show the comparison between our perturbation theory with Barash’s exact result [1] for the torque between uniaxial materials, whose optical axes make an angle  $\theta$  with respect to each other and are perpendicular to  $\hat{\mathbf{n}}$ , in Fig. 1. We generated “uniaxial” materials using dielectric function of BP<sup>(XY)</sup> and BP<sup>(XZ)</sup> after setting the dielectric component in the direction  $\hat{\mathbf{n}}$  of the system equal to one of the in-planar dielectric components,  $\varepsilon^y = \varepsilon^z$ . We compare our results for two cases: the interaction between two nonidentical materials, and the interaction between two identical materials. The leading order perturbation theory matches with the exact theory excellently for the case of the interaction between the identical materials. For the interaction between nonidentical materials the relative percentage error remains within 0.5-5.5% for most of the test range of separation distances 1-100 nm. The relative error grows large near the separation distance where the torque changes sign as we are dividing by a very small value. The numerical evaluation of the perturbative calculation performs faster than the exact calculation. The leading order torque with actual data for the  $z$  component is also shown for comparison. The inclusion of  $\varepsilon^z$  component not only changes the magnitude of the torque but can also shift the critical separation distance for a fixed angle  $\theta$ .

We have also verified and compared results for actual uniaxial materials, like calcite and quartz, using the dielectric tensor data given in [2]. The perturbative parameter for quartz is of the order of  $10^{-3}$  while that for calcite remains below 0.1 (which is zero at two characteristic frequencies) for all frequencies. As predicted, the interaction between calcite and quartz leads to a sign-reversal in the torque between 1.3-1.4  $\mu\text{m}$ , which suggests that the sign-reversal

behavior is governed by the smaller of the two characteristic frequencies for calcite. The two theories match excellently with the percentage relative error staying within 1% between 1 to  $2\mu\text{m}$  except close to the sign-reversal distance, where the value of the torque itself is small.

## DIELECTRIC FUNCTION CALCULATION USING DENSITY FUNCTIONAL THEORY

The optical properties of BP and 2D-P are computed within the independent particle approximation using the Vienna Ab-initio Simulation Package (VASP). Herein, the structures are relaxed with the optB88-vdW functional [3] to treat the exchange-correlation term taking into account the layered configuration of the material. The optoelectronic properties are calculated for the optB88-vdW structures employing the revised Heyd-Scuseria-Ernzerhof (HSE) screened hybrid functional [4]. The cut-off energy for the plane-wave basis sets is set at 600 eV and 325 eV for the relaxation and optical calculations respectively.  $8 \times 8 \times 10$  and  $14 \times 14 \times 1$   $\Gamma$ -centered Monkhorst-Pack k-grids [5] are used in the Brillouin-zone integrations for BP and 2D-P, respectively. With the selected computational setup, the computed band gap energies of BP and 2D-P are 0.38 and 1.52 eV, respectively. These results are consistent with the previously reported results [6]. Since the original framework for optical calculations within the independent particle approximation is developed for 3-dimensional systems, the computed frequency-dependent dielectric function of phosphorene is scaled to the volume of a single layer. The volume correction is carried out with the assumption that the single layer corresponds to a thickness of  $d = 5.37 \text{ \AA}$ , which is half the length of the long direction of the bulk conventional unit cell. The bulk conventional unit cell is schematically depicted in the inset of Fig. 1 in the main text. It may be mentioned that different choices of the layer thickness do not alter our torque results.

- 
- [1] Yu. S. Barash, “Moment of van der Waals forces between anisotropic bodies,” *Radiophys. Quantum Electron.* **21**, 1138 (1978), [Translated from: *Izv. VUZ. Radiofizika* **21**, 1637 (1978)].
  - [2] J. N. Munday, D. Iannuzzi, Yu. S. Barash, and F. Capasso, “Torque on birefringent plates induced by quantum fluctuations,” *Phys. Rev. A* **71**, 042102 (2005).
  - [3] J. Klimeš, D. R. Bowler, and A. Michaelides, “Chemical accuracy for the van der Waals density functional,” *J. Phys. Condens. Matter* **22**, 022201 (2010); “van der Waals density functionals applied to solids,” *Phys. Rev. B* **83**, 195131 (2011).
  - [4] A. V. Krukau, O. A. Vydrov, A. F. Izmaylov, and G. E. Scuseria, “Influence of the exchange screening parameter on the performance of screened hybrid functionals,” *J. Chem. Phys.* **125**, 224106 (2006).
  - [5] H. J. Monkhorst and J. D. Pack, “Special points for Brillouin-zone integrations,” *Phys. Rev. B* **13**, 5188 (1976).
  - [6] O. I. Malyi, K. Sopiha, I. Radchenko, P. Wu, and C. Persson, “Tailoring electronic properties of multilayer phosphorene by siliconization,” *Phys. Chem. Chem. Phys.* (2017), 10.1039/c7cp06196j.
